# Supplementary material for: Harnessing TI Feeds for Exploitation Detection
Source: arXiv:2409.07709 source file (2024-09-12)
Supplement: Supplementary file 2 [file appendix1.tex]

\section{Rule mining for Ground truth} \label{sec:ruleminingappendix}

Table~\ref{table: full-rules} reports the  list of top  most frequent  rules used for labeling exploitation  events. Such rules were mined using the \emph{apriori} algorithm, based on a set of manually labeled events. In the table, for each rule we indicate the number of tags involved in the rule,  its confidence and lift. 

%\tiny
%\setlength\LTleft{-1em}
%\setlength\LTright{0pt}
\begin{longtable}{|p{\columnwidth}|r|r|r|}
\caption{Top 
most frequent rules labeling exploitation.} \label{tab:long} \\

\hline \multicolumn{1}{|c|}{\textbf{Rules}} & \multicolumn{1}{c|}{\textbf{Tags}} & \multicolumn{1}{c|}{\textbf{Confidence}} & \multicolumn{1}{c|}{\textbf{Lift}}\\ \hline 
\endfirsthead

\multicolumn{4}{c}%
{{\bfseries \tablename\ \thetable{} -- continued from previous page}} \\
\hline \multicolumn{1}{|c|}{\textbf{Rules}} & \multicolumn{1}{c|}{\textbf{Tags}} & \multicolumn{1}{c|}{\textbf{Confidence Score}} & \multicolumn{1}{c|}{\textbf{Lift Score}}\\ \hline 
\endhead

\hline \multicolumn{4}{|r|}{{Continued on next page}} \\ \hline
\endfoot
\hline
\hline \multicolumn{4}{|r|}{{End of table}} \\ \hline
\endlastfoot

\hline
(threat:ransomware)+(malware\_classification:malware-category="ransomware")                                                                                                       & 2                                            & 1.00                                  & 3.58                                                          \\ 
\hline
(circl:incident-classification="spam")+(malware\_classification:malware-category="trojan")                                                                                        & 2                                            & 1.00                                  & 3.58                                                          \\ 
\hline
(veris:confidence="none")+(cssa:origin="other")+(malware\_classification:malware-category="ransomware")+(cssa:sharing-class="tier-0")                                             & 4                                            & 1.00                                  & 3.58                                                          \\ 
\hline
(cssa:origin="other")+(malware\_classification:malware-category="ransomware")+(cssa:sharing-class="tier-0")                                                                       & 3                                            & 1.00                                  & 3.58                                                          \\ 
\hline
(veris:confidence="none")+(cssa:origin="other")+(malware\_classification:malware-category="ransomware")                                                                           & 3                                            & 1.00                                  & 3.58                                                          \\ 
\hline
(veris:confidence="none")+(malware\_classification:malware-category="ransomware")+(cssa:sharing-class="tier-0")                                                                   & 3                                            & 1.00                                  & 3.58                                                          \\ 
\hline
(veris:confidence="none")+(malware\_classification:malware-category="ransomware")                                                                                                 & 2                                            & 1.00                                  & 3.58                                                          \\ 
\hline
(cssa:origin="other")+(malware\_classification:malware-category="ransomware")                                                                                                     & 2                                            & 1.00                                  & 3.58                                                          \\ 
\hline
(malware\_classification:malware-category="ransomware")+(cssa:sharing-class="tier-0")                                                                                             & 2                                            & 1.00                                  & 3.58                                                          \\ 
\hline
(ms-caro-malware:malware-platform="macos\_x")                                                                                                                                     & 1                                            & 1.00                                  & 3.43                                                          \\ 
\hline
(type:osint)+(cssa:origin="other")+(malware\_classification:malware-category="ransomware")+(cssa:sharing-class="tier-0")                                                          & 4                                            & 1.00                                  & 3.58                                                          \\ 
\hline
(veris:confidence="none")+(type:osint)+(cssa:origin="other")+(malware\_classification:malware-category="ransomware")                                                              & 4                                            & 1.00                                  & 3.58                                                          \\ 
\hline
(type:osint)+(veris:confidence="none")+(malware\_classification:malware-category="ransomware")+(cssa:sharing-class="tier-0")                                                      & 4                                            & 1.00                                  & 3.58                                                          \\ 
\hline
(type:osint)+(cssa:origin="other")+(malware\_classification:malware-category="ransomware")                                                                                        & 3                                            & 1.00                                  & 3.58                                                          \\ 
\hline
(type:osint)+(malware\_classification:malware-category="ransomware")+(cssa:sharing-class="tier-0")                                                                                & 3                                            & 1.00                                  & 3.58                                                          \\ 
\hline
(apt)+(kill-chain:installation)+(kill-chain:command and control)                                                                                                                  & 3                                            & 1.00                                  & 3.58                                                          \\ 
\hline
(type:osint)+(veris:confidence="none")+(malware\_classification:malware-category="ransomware")                                                                                    & 3                                            & 1.00                                  & 3.58                                                          \\ 
\hline
(veris:asset:variety="s - scada")+(circl:topic="industry")                                                                                                                        & 2                                            & 1.00                                  & 3.58                                                          \\ 
\hline
(circl:incident-classification="system-compromise")+(circl:incident-classification="vulnerability")                                                                               & 2                                            & 1.00                                  & 3.58                                                          \\ 
\hline
(apt)+(kill-chain:installation)                                                                                                                                                   & 2                                            & 1.00                                  & 3.58                                                          \\ 
\hline
(malspam)+(banker)                                                                                                                                                                & 2                                            & 1.00                                  & 3.58                                                          \\ 
\hline
(apt)+(kill-chain:command and control)                                                                                                                                            & 2                                            & 1.00                                  & 3.58                                                          \\ 
\hline
(veris:asset:variety="s - scada")                                                                                                                                                 & 1                                            & 1.00                                  & 3.43                                                          \\ 
\hline
(veris:asset:variety="u - pos terminal")                                                                                                                                          & 1                                            & 1.00                                  & 3.43                                                          \\ 
\hline
(enisa:nefarious-activity-abuse="spear-phishing-attacks")                                                                                                                         & 1                                            & 1.00                                  & 3.43                                                          \\ 
\hline
(circl:incident-classification="spam")+(threat:ransomware)+(malware\_classification:malware-category="ransomware")                                                                & 3                                            & 1.00                                  & 3.58                                                          \\ 
\hline
(circl:incident-classification="phishing")+(malware\_classification:malware-category="ransomware")+(phishing)                                                                     & 3                                            & 1.00                                  & 3.58                                                          \\ 
\hline
(circl:incident-classification="phishing")+(enisa:nefarious-activity-abuse="phishing-attacks")+(phishing)                                                                         & 3                                            & 1.00                                  & 3.58                                                          \\ 
\hline
(cybercrime)+(sectorfinancial)+(kill-chain:installation)                                                                                                                          & 3                                            & 1.00                                  & 3.58                                                          \\ 
\hline
(apt)+(ncsc-nl-nds:search="historic")+(osint)                                                                                                                                     & 3                                            & 1.00                                  & 3.58                                                          \\ 
\hline
(malware\_classification:malware-category="ransomware")+(circl:incident-classification="malware")+(malware\_classification:malware-category="worm")                               & 3                                            & 1.00                                  & 3.58                                                          \\ 
\hline
(circl:incident-classification="phishing")+(circl:topic="finance")+(circl:incident-classification="malware")                                                                      & 3                                            & 1.00                                  & 3.58                                                          \\ 
\hline
(threat:ransomware)+(ecsirt:malicious-code="ransomware")+(malware\_classification:malware-category="ransomware")                                                                  & 3                                            & 1.00                                  & 3.58                                                          \\ 
\hline
(sectorfinancial)+(kill-chain:installation)                                                                                                                                       & 2                                            & 1.00                                  & 3.58                                                          \\ 
\hline
(malware\_classification:malware-category="ransomware")+(malware\_classification:malware-category="worm")                                                                         & 2                                            & 1.00                                  & 3.58                                                          \\ 
\hline
(osint)+(ncsc-nl-nds:search="historic")                                                                                                                                           & 2                                            & 1.00                                  & 3.58                                                          \\ 
\hline
(type:osint)+(veris:action:malware:variety="ransomware")                                                                                                                          & 2                                            & 1.00                                  & 3.58                                                          \\ 
\hline
(veris:actor:motive="financial")+(circl:topic="finance")                                                                                                                          & 2                                            & 1.00                                  & 3.58                                                          \\ 
\hline
(threat:ransomware)                                                                                                                                                               & 1                                            & 0.86                                  & 2.94                                                          \\ 
\hline
(circl:incident-classification="phishing")+(phishing)                                                                                                                             & 2                                            & 0.83                                  & 2.98                                                          \\ 
\hline
(circl:incident-classification="phishing")+(enisa:nefarious-activity-abuse="phishing-attacks")                                                                                    & 2                                            & 0.83                                  & 2.98                                                          \\ 
\hline
(malware\_classification:malware-category="ransomware")+(phishing)                                                                                                                & 2                                            & 0.83                                  & 2.98                                                          \\ 
\hline
(enisa:nefarious-activity-abuse="phishing-attacks")                                                                                                                               & 1                                            & 0.83                                  & 2.86                                                          \\ 
\hline
(veris:actor:motive="financial")                                                                                                                                                  & 1                                            & 0.83                                  & 2.86                                                          \\ 
\hline
(threat:snake)                                                                                                                                                                    & 1                                            & 0.83                                  & 2.86                                                          \\ 
\hline
(circl:incident-classification="phishing")+(malware\_classification:malware-category="trojan")                                                                                    & 2                                            & 0.80                                  & 2.86                                                          \\ 
\hline
(type:osint)+(ecsirt:malicious-code="ransomware")                                                                                                                                 & 2                                            & 0.80                                  & 2.86                                                          \\ 
\hline
(malspam)+(nymaim)                                                                                                                                                                & 2                                            & 0.80                                  & 2.86                                                          \\ 
\hline
(type:osint)+(threat:snake)                                                                                                                                                       & 2                                            & 0.80                                  & 2.86                                                          \\ 
\hline
(ncsc-nl-nds:search="historic")+(ncsc-nl-ndn:feed="selected")                                                                                                                     & 2                                            & 0.80                                  & 2.86                                                          \\ 
\hline
(apt)+(osint)                                                                                                                                                                     & 2                                            & 0.80                                  & 2.86                                                          \\ 
\hline
(relcircl)                                                                                                                                                                        & 1                                            & 0.80                                  & 2.74                                                          \\ 
\hline
(circl:topic="finance")+(circl:incident-classification="malware")                                                                                                                 & 2                                            & 0.75                                  & 2.68                                                          \\ 
\hline
(malware\_classification:malware-category="spyware")                                                                                                                              & 1                                            & 0.75                                  & 2.57                                                          \\ 
\hline
(veris:action:social:target="finance")+(circl:topic="finance")                                                                                                                    & 2                                            & 0.75                                  & 2.68                                                          \\ 
\hline
(certsi:critical-sector="energy")                                                                                                                                                 & 1                                            & 0.75                                  & 2.57                                                          \\ 
\hline
(danabot)                                                                                                                                                                         & 1                                            & 0.75                                  & 2.57                                                          \\ 
\hline
(threat type:rat)                                                                                                                                                                 & 1                                            & 0.75                                  & 2.57                                                          \\ 
\hline
(sectorfinancial)                                                                                                                                                                 & 1                                            & 0.75                                  & 2.57                                                          \\ 
\hline
(type:osint)+(malware\_classification:malware-category="ransomware")                                                                                                              & 2                                            & 0.72                                  & 2.58                                                          \\ 
\hline
(circl:incident-classification="spam")                                                                                                                                            & 1                                            & 0.71                                  & 2.45                                                          \\ 
\hline
(type:osint)+(circl:topic="finance")                                                                                                                                              & 2                                            & 0.71                                  & 2.55                                                          \\ 
\hline
(circl:incident-classification="phishing")+(circl:incident-classification="malware")                                                                                              & 2                                            & 0.71                                  & 2.55                                                          \\ 
\hline
(malware\_classification:malware-category="botnet")                                                                                                                               & 1                                            & 0.71                                  & 2.45                                                          \\ 
\hline
(veris:action:social:variety="phishing")                                                                                                                                          & 1                                            & 0.71                                  & 2.45                                                          \\ 
\hline
(circl:topic="finance")                                                                                                                                                           & 1                                            & 0.70                                  & 2.41                                                          \\ 
\hline
(ncsc-nl-nds:search="historic")                                                                                                                                                   & 1                                            & 0.70                                  & 2.40  
\label{table: full-rules}
\end{longtable}

\end{appendix}
